# Supplementary material for: LinVT: Empower Your Image-level Large Language Model to Understand Videos
Source: arXiv:2412.05185 source file (2024-12-11)
Supplement: Supplementary file 1 [file suppl_ablation_svr_tta.tex]

\begin{table*}[h!]
\centering
\resizebox{\textwidth}{!}{%
\begin{tabular}{cc|ccccccccccc}
\hline
SVR & TTA & {MVB} & {MMB-V} & {V-MME} & {LongVB} & {N-QA} & {EgoS} & {MVD-QA} & {MTT-QA} & {Act-QA} & {TGIF-QA}\\
\hline
& & 41.6 & 0.55 & 30.5 / 30.1 & 31.0 & 40.7 & 29.8 &  35.4 / 1.8 & 24.1 / 1.2 & 20.3 / 1.6 & 33.2 / 1.5 \\
\checkmark & & 60.3 & 1.12 & 45.7 / 46.1 & 46.2 & 67.1 & 51.4 & 67.5 / 3.4 & 52.7 / 2.7 & 46.2 / 2.9 & 68.9 / 3.6\\
& \checkmark & 58.7 & 1.03 & 45.4 / 45.7 & 44.8 & 65.1 & 50.2 & 64.1 / 3.2 & 50.3 / 2.4 & 41.6 / 2.6 & 66.9 / 3.2\\
\checkmark & \checkmark & \textbf{62.5} & \textbf{1.22} & \textbf{48.4} / \textbf{49.2} & \textbf{49.7} & \textbf{71.1} & \textbf{55.9} & \textbf{71.2} / \textbf{3.8} & \textbf{55.3} / \textbf{3.0} & \textbf{47.5} / \textbf{3.1} & \textbf{71.1} / \textbf{3.9} \\
\hline
\end{tabular}%
}
% \vspace{-1em}
\caption{
Ablation studies on the effectiveness of SVR and TTA. The image-LLM used in this experiment is Mipha-1.6B. We include the result of the baseline without the proposed LinVT modules compared to \cref{tab:sub_modules}.}
\label{tab:suppl_sub_modules}
\end{table*}
