# Supplementary material for: LinVT: Empower Your Image-level Large Language Model to Understand Videos
Source: arXiv:2412.05185 source file (2024-12-11)
Supplement: Supplementary file 2 [file suppl_video_zeroshot.tex]

\begin{table*}[h!]
\centering

\resizebox{\textwidth}{!}{
\begin{tabular}{l|c|cccc}
\hline
{Method} & {Size} & MVD-QA & MTT-QA & Act-QA & TGIF-QA \\
\hline
BLIP-3-Video~\cite{ryoo2024xgen} & 4B & {77.7 / 4.2} & {60.0 / 3.6} & {\closeruline{55.7} / \closeruline{3.5}} & {76.5 / \textbf{4.3}} \\
\hline
\rowcolor[HTML]{EFEFEF} 
LinVT-BLIP-$3^*$ & 4B & \closeruline{78.1} / \closeruline{4.3} & \closeruline{60.3} / \closeruline{3.8} & 55.6 / \closeruline{3.5} & \closeruline{76.9} / \textbf{4.3} \\
\rowcolor[HTML]{EFEFEF} 
LinVT-BLIP-3     & 4B & \textbf{79.1} / \textbf{4.4} & \textbf{61.5} / \textbf{3.9} & \textbf{58.9} / \textbf{3.6} & \textbf{78.7} / \textbf{4.3} \\
\hline
\end{tabular}%
}
\vspace{-0.5em}
\caption{
Comparison with BLIP-3-Video~\cite{ryoo2024xgen} on four zero-shot video QA datasets. Particularly, * indicates the model trained on the same data as BLIP-3-Video. The best results are in \textbf{bold} and second best \ul{underlined}.
}
\label{tab:suppl_res_openend}
\end{table*}
